# Supplementary material for: Towards Personalized Prostate Cancer Therapy Using Delta-Reachability Analysis
Source: arXiv:1410.7346 source file (2015-05-19)
Supplement: Supplementary file 1 [file appendix.tex]

\newpage
\section*{Appendix}

\subsection*{$\lrf$-Formulas and $\delta$-Decidability}

We will use a logical language over the real numbers that allows arbitrary {\em computable real functions}. We write $\lrf$ to represent this language. Intuitively, a real function is computable if it can be numerically simulated up to an arbitrary precision. For the purpose of this paper, it suffices to know that almost all the functions that are needed in describing hybrid systems are Type 2 computable (i.e. computable by a Type-2 machine), such as polynomials, exponentiation, logarithm, trigonometric functions, and solution functions of Lipschitz-continuous ordinary differential equations.

More formally, $\lrf = \langle \mathcal{F}, > \rangle$ represents the first-order signature over the reals with the set $\mathcal{F}$ of computable real functions, which contains all the functions mentioned above. Note that constants are included as 0-ary functions. $\lrf$-formulas are evaluated in the standard way over the structure $\mathbb{R}_{\mathcal{F}}= \langle \mathbb{R}, \mathcal{F}^{\mathbb{R}}, >^{\mathbb{R}}\rangle$. It is not hard to see that  we can put any $\lrf$-formula in a normal form, such that its atomic formulas are of the form $t(x_1,...,x_n)>0$ or $t(x_1,...,x_n)\geq 0$, with $t(x_1,...,x_n)$ composed of functions in $\mathcal{F}$. To avoid extra preprocessing of formulas, we can explicitly define $\mathcal{L}_{\mathcal{F}}$-formulas as follows.

\begin{definition}[$\lrf$-Formulas]
Let $\mathcal{F}$ be a collection of computable real functions. We define:
\begin{align*}
t& := x \; | \; f(t(\vec x)), \mbox{ where }f\in \mathcal{F} \mbox{ (constants are 0-ary functions)};\\
\varphi& := t(\vec x)> 0 \; | \; t(\vec x)\geq 0 \; | \; \varphi\wedge\varphi
\; | \; \varphi\vee\varphi \; | \; \exists x_i\varphi \; |\; \forall x_i\varphi.
\end{align*}
In this setting $\neg\varphi$ is regarded as an inductively defined operation
which replaces atomic formulas $t>0$ with $-t\geq 0$, atomic formulas $t\geq 0$
with $-t>0$, switches $\wedge$ and $\vee$, and switches $\forall$ and $\exists$.
\end{definition}

\begin{definition}[Bounded $\lrf$-Sentences]
We define the bounded quantifiers $\exists^{[u,v]}$ and $\forall^{[u,v]}$ as
$\exists^{[u,v]}x.\varphi =_{df}\exists x. ( u \leq x \land x \leq v \wedge
\varphi)$ and $
\forall^{[u,v]}x.\varphi =_{df} \forall x. ( (u \leq x \land x \leq v)
\rightarrow \varphi)$
where $u$ and $v$ denote $\lrf$ terms, whose variables only
contain free variables in $\varphi$ excluding $x$. A {\em bounded $\lrf$-sentence} is
$$Q_1^{[u_1,v_1]}x_1\cdots Q_n^{[u_n,v_n]}x_n\;\psi(x_1,...,x_n),$$
where $Q_i^{[u_i,v_i]}$ are bounded quantifiers, and $\psi(x_1,...,x_n)$ is
quantifier-free.
\end{definition}

\begin{definition}[$\delta$-Variants]\label{variants}
Let $\delta\in \mathbb{Q}^+\cup\{0\}$, and $\varphi$ an
$\lrf$-formula
$$\varphi: \ Q_1^{I_1}x_1\cdots Q_n^{I_n}x_n\;\psi[t_i(\vec x, \vec y)>0;
t_j(\vec x, \vec
y)\geq 0],$$ where $i\in\{1,...k\}$ and $j\in\{k+1,...,m\}$. The {\em
$\delta$-weakening} $\varphi^{\delta}$ of $\varphi$ is
defined as the result of replacing each atom $t_i > 0$ by $t_i >
-\delta$ and $t_j \geq 0$ by $t_j \geq -\delta$:
$$\varphi^{\delta}:\ Q_1^{I_1}x_1\cdots Q_n^{I_n}x_n\;\psi[t_i(\vec x, \vec
y)>-\delta; t_j(\vec x,
\vec y)\geq -\delta].$$
It is clear that $\varphi\rightarrow\varphi^{\delta}$~(see \cite{gao12b}).
\end{definition}
In~\cite{gao12a}, we have proved that the following $\delta$-decision problem is decidable, which is the basis of our framework.

\textbf{Theorem 1 $\delta$-Decidability \cite{gao12a}}
%\begin{theorem}[$\delta$-Decidability \cite{gao12a}]\label{delta-decide} 
Let $\delta\in\mathbb{Q}^+$ be
arbitrary. There is an algorithm which, given any bounded $\lrf$-sentence $\varphi$,
correctly returns one of the following two answers:
\begin{itemize}
\item $\delta$-$\mathsf{True}$: $\varphi^{\delta}$ is true.
\item $\mathsf{False}$: $\varphi$ is false.
\end{itemize}
When the two cases overlap, either answer is correct.
%\end{theorem}

The following theorem states the (relative) complexity of the $\delta$-decision problem.
A bounded $\Sigma_n$ sentence is a bounded $\lrf$-sentence with $n$ alternating quantifier blocks 
starting with $\exists$. 

\textbf{Theorem 2 Complexity \cite{gao12b}}
%\begin{theorem}[Complexity \cite{gao12b}]\label{compmain}
Let $S$ be a class of $\lrf$-sentences, such that for any $\varphi$ in $S$, the terms in $\varphi$ are in Type 2 complexity class $\mathsf{C}$. Then, for any $\delta\in \mathbb{Q}^+$, the $\delta$-decision problem for bounded $\Sigma_n$-sentences in $S$ is in $\mathsf{(\Sigma_n^P)^C}$.
%\end{theorem}

Basically, the theorem says that increasing the number of quantifier alternations will in general increase 
the complexity of the problem, unless $\mathsf{P}=\mathsf{NP}$ (recall that $\mathsf{\Sigma_0^P}=\mathsf{P}$ 
and $\mathsf{\Sigma_1^P}=\mathsf{NP}$).
This result can specialized for specific families of functions. For example, with polynomially-computable 
functions, the $\delta$-decision problem for bounded $\Sigma_n$-sentences is $\mathsf{(\Sigma_n^P)}$-complete.
For more details and results we again point the interested reader to \cite{gao12b}.

\subsection*{Delta-Decisions for Hybrid Models}

Now we state the encoding for hybrid models. Recall that hybrid automata generalize finite-state
automata by permitting continuous-time evolution (or {\em flow}) in each discrete state (or {\em mode}). 
Also, in each mode an {\em invariant} must be satisfied by the flow, and mode switches are controlled
by {\em jump} conditions.

\begin{definition}[$\lrf$-Representations of Hybrid Automata]\label{lrf-definition}
A hybrid automaton in $\lrf$-representation is a tuple
\begin{multline*}
H = \langle X, Q, \{{\flow}_q(\vec x, \vec y, t): q\in Q\},\{\inv_q(\vec x): q\in Q\},\\
\{\jump_{q\rightarrow q'}(\vec x, \vec y): q,q'\in Q\},\{\init_q(\vec x): q\in Q\}\rangle
\end{multline*}
where $X\subseteq \mathbb{R}^n$ for some $n\in \mathbb{N}$, $Q=\{q_1,...,q_m\}$ is a finite set of modes, and the other components are finite sets of quantifier-free $\lrf$-formulas.
\end{definition}

%\begin{example}[Nonlinear Bouncing Ball]
%The bouncing ball is a standard hybrid system model. It can be $\lrf$-represented in the following way:
%\begin{itemize}
%\item $X = \mathbb{R}^2$ and $Q = \{q_u, q_d\}$. We use $q_u$ to represent bounce-back mode and $q_d$ the falling mode.
%\item $\flow = \{\flow_{q_u}(x_0, v_0, x_t, v_t, t), \flow_{q_d}(x_0, v_0, x_t, v_t, t)\}$. We use $x$ to denote the height of the ball and $v$ its velocity. Instead of using time derivatives, we can directly write the flows as integrals over time, using $\lrf$-formulas:
%\begin{itemize}
%\item $\flow_{q_u}(x_0, v_0, x_t, v_t, t)$ defines the dynamics in the bounce-back phase:
%$$(x_t = x_0 + \int_0^{t} v(s) ds) \wedge (v_t = v_0 + \int_0^t g(1-\beta v(s)^2) ds)$$
%\item $\flow_{q_d}(x_0, v_0, x_t, v_t, t)$ defines the dynamics in the falling phase:
%$$(x_t = x_0 + \int_0^{t} v(s) ds) \wedge (v_t = v_0 + \int_0^t g(1+\beta v(s)^2) ds)$$
%\end{itemize}where
%$\beta$ is a constant. Again, note that the integration terms define Type 2 computable functions.
%\item $\jump = \{\jump_{q_u \rightarrow q_d} (x, v, x', v'), \jump_{q_d \rightarrow q_u} (x, v, x', v')\}$ where
%\begin{itemize}
%\item $\jump_{q_u \rightarrow q_d} (x, v, x', v')$ is $(v= 0 \wedge x' = x \wedge v' = v)$.
%\item $\jump_{q_d \rightarrow q_u} (x, v, x', v')$ is $(x= 0 \wedge v' = \alpha v\wedge x'=x)$,  for some constant $\alpha$.
%\end{itemize}
%\item $\init_{q_d}$ is $(x=10 \wedge v=0)$ and $\init_{q_u}$ is $\bot$.
%\item $\inv_{q_d}$ is $(x>=0 \wedge v>=0)$ and $\inv_{q_u}$ is $(x>=0 \wedge v<=0)$.
%\end{itemize}
%\end{example}

We now show the encoding of bounded reachability, which is used for encoding the parameter synthesis
problem. We want to decide whether a given 
hybrid system reaches a particular region of its state space after following a (bounded) number
of discrete transitions, \ie, jumps. First, we need to define auxiliary formulas used
for ensuring that a particular mode is picked at a certain step.

\begin{definition}
Let $Q = \{q_1,...,q_m\}$ be a set of modes. For any $q\in Q$, and $i\in\mathbb{N}$, use  $b_{q}^i$ to represent a Boolean variable. We now define
$$\enforce_Q(q,i) = b^i_{q} \wedge \bigwedge_{p\in Q\setminus\{q\}}\neg b^{i}_{p}$$
$$\enforce_Q(q, q',i) = b^{i}_{q}\wedge \neg b^{i+1}_{q'} \wedge \bigwedge_{p\in Q\setminus\{q\}} \neg b^i_{p} \wedge \bigwedge_{p'\in Q\setminus\{q'\}} \neg b^{i+1}_{p'}$$
We omit the subscript $Q$ when the context is clear.\end{definition}

We can now define the following formula that checks whether a {\em goal} region of the automaton
state space is reachable after exactly $k$ discrete transitions. We first state 
the simpler case of a hybrid system without invariants.

\begin{definition}[$k$-Step Reachability, Invariant-Free Case]
Suppose $H$ is an invariant-free hybrid automaton, $U$ a subset of its state space represented by $\goal$,
and $M>0$. The formula $\reach_{H,U}(k,M)$ is defined as:
\begin{eqnarray*}
%\reach^{k,M}(H,U) &:=&
& &\exists^X \vec x_{0} \exists^X\vec x_{0}^t\cdots \exists^X \vec x_{k}\exists^X\vec x_{k}^t\exists^{[0,M]}t_0\cdots \exists^{[0,M]}t_k.\\
& &\bigvee_{q\in Q} \Big(\init_{q}(\vec x_{0})\wedge \flow_{q}(\vec x_{0}, \vec x_{0}^t, t_0)\wedge \enforce(q,0)\Big)\\
\wedge & & \bigwedge_{i=0}^{k-1}\bigg( \bigvee_{q, q'\in Q} \Big(\jump_{q\rightarrow q'}(\vec x_{i}^t, \vec x_{i+1})\wedge \enforce(q,q',i)\\
& & \wedge\flow_{q'}(\vec x_{i+1}, \vec x_{i+1}^t, t_{i+1})\wedge \enforce(q',i+1)\Big)\bigg)\\
\wedge & &\bigvee_{q\in Q} (\goal_q(\vec x_{k}^t)\wedge \enforce(q,k))
\end{eqnarray*}
where $\exists^X x$ is a shorthand for $\exists x\in X$.
\end{definition}
Intuitively, the trajectories start with some initial state satisfying $\init_q(\vec x_{0})$ for some $q$. 
Then, in each step the trajectory follows $\flow_q(\vec x_{i}, \vec x_{i}^t, t)$ and makes a continuous flow from $\vec x_i$ to $\vec x_i^t$ after time $t$. When the automaton makes a $\jump$ from mode $q'$ to $q$, it resets variables following $\jump_{q'\rightarrow q}(\vec x_{k}^t, \vec x_{k+1})$. The auxiliary $\enforce$ formulas ensure that picking $\jump_{q\rightarrow q'}$ in the $i$-the step enforces picking $\flow_q'$ in the $(i+1)$-th step.

When the invariants are not trivial, we need to ensure that for all the time points along a continuous flow, the invariant condition holds. We need to universally quantify over time, and the encoding is as follows:

\begin{definition}[$k$-Step Reachability, Nontrivial Invariant]\label{br2}
Suppose $H$ contains invariants, and $U$ is a subset of the state space represented by $\goal$. The $\lrf$-formula $\reach_{H,U}(k,M)$ is defined as:
\begin{eqnarray*}
& &\exists^X \vec x_{0} \exists^X\vec x_{0}^t\cdots \exists^X \vec x_{k}\exists^X\vec x_{k}^t \exists^{[0,M]}t_0\cdots \exists^{[0,M]}t_k.\\
& &\bigvee_{q\in Q} \Big(\init_{q}(\vec x_{0})\wedge \flow_{q}(\vec x_{0}, \vec x_{0}^t, t_0)\wedge \enforce(q,0)\\
& &\hspace{0cm} \wedge \forall^{[0,t_0]}t\forall^X\vec x\;(\flow_{q}(\vec x_{0}, \vec x, t)\rightarrow \inv_{q}(\vec x))\Big) \\
\wedge & &\bigwedge_{i=0}^{k-1}\bigg( \bigvee_{q, q'\in Q} \Big(\jump_{q\rightarrow q'}(\vec
x_{i}^t, \vec x_{i+1})\wedge \flow_{q'}(\vec x_{i+1}, \vec x_{i+1}^t, t_{i+1})\\
& & \wedge \enforce(q,q',i)  \wedge\enforce(q',i+1)\\
& & \wedge \forall^{[0,t_{i+1}]}t\forall^X\vec x\;(\flow_{q'}(\vec x_{i+1}, \vec x,
t)\rightarrow \inv_{q'}(\vec x)) )\Big)\bigg)\\
\wedge & &\bigvee_{q\in Q} (\goal_q(\vec x_{k}^t)\wedge \enforce(q,k)).
\end{eqnarray*}
\end{definition}

The extra universal quantifier for each continuous flow expresses the requirement that for all the time points between the initial and ending time point ($t\in[0,t_i+1]$) in a flow, the continuous variables $\vec x$ must take values that satisfy the invariant conditions $\inv_q(\vec x)$.
